# Supplementary material for: Hyperfine-mediated transitions between electronic spin-1/2 levels of transition metal defects in SiC
Source: arXiv:2104.12433 ancillary file (2021-09-02)
Supplement: Supplementary file 1 [file Supplementary.pdf]

# Supplementary Information for *Hyperfine-mediated transitions between electronic spin-1/2 levels of transition metal defects in SiC*

Carmem M. Gilardoni,[1,*] Irina Ion,[1] Freddie Hendriks,[1]
Michael Trupke,[2] and Caspar H. van der Wal[1,†]

[1]*Zernike Institute for Advanced Materials, University of Groningen, NL-9747AG Groningen, The Netherlands*

[2]*Vienna Center for Quantum Science and Technology, University of Vienna, VCQ, Boltzmanngasse 5,1090 Vienna, Austria*

(Dated: Version of April 26, 2021)

* c.maia.gilardoni@rug.nl

† c.h.van.der.wal@rug.nl

## I. MATRIX REPRESENTATION OF CRYSTAL FIELD HAMILTONIAN

A TM defect with one active spin in the $d$-orbitals of the TM core corresponds to an electron with spin $s = 1/2$ and orbital angular momentum $l = 2$ (from the $d$-orbitals). Spatially, these states are affected only by the combination of the cubic and trigonal crystal fields. If we disregard the effect of bonding and assume that these states are well-isolated from other core orbitals of the TM impurity due to the Coulomb interaction with the nucleus, the basis states for the $d$ orbitals form a complete basis set to describe the electronic wavefunction.

In free space, the 5 spherical harmonics $Y_2^m$ that span the $d$ orbital states are degenerate. They form a 5-dimensional irreducible representation (irrep) of the full rotation group SO(3). The $d$ orbital states can equally well be described by cubic harmonics, which can be written in terms of spherical harmonics as

$$\left|z^2\right\rangle = Y_2^0 \tag{s1}$$

$$|xz\rangle = \left(Y_2^{-1} - Y_2^1\right)/\sqrt{2} \tag{s2}$$

$$|yz\rangle = i\left(Y_2^{-1} + Y_2^1\right)/\sqrt{2} \tag{s3}$$

$$|xy\rangle = i\left(Y_2^{-2} - Y_2^2\right)/\sqrt{2} \tag{s4}$$

$$\left|x^2 - y^2\right\rangle = \left(Y_2^{-2} + Y_2^2\right)/\sqrt{2} \tag{s5}$$

In hexagonal SiC, the predominant symmetry at the TM defect is tetrahedral at a silicon substitutional site [1]. The crystal field, which is the potential due to the surrounding crystal with which the $d$ electron interacts, reflects this symmetry. The 5 spherical harmonics do not form an irrep of the cubic symmetry groups. Therefore they are split by the crystal field into irreps of these groups. How the states are split can be calculated using the theory of characters of representations. For tetrahedral symmetry, the 5 states of the $d$ orbitals split into an orbital doublet and an orbital triplet. The doublet is composed of the cubic harmonics $|x'^2 - y'^2\rangle$ and $|z'^2\rangle$, and the triplet by $|x'y'\rangle$, $|x'z'\rangle$ and $|y'z'\rangle$. The primed cubic harmonics indicate the direction of the cartesian coordinates in these functions, and are such that the $z'$-axis coincides with a 4-fold rotational axis of the cubic field (between two of the tetrahedral bonds). In the basis $cb'$ defined by the primed cubic harmonics, $cb' = \{|z'^2\rangle, |x'z'\rangle, |y'z'\rangle, |x'y'\rangle, |x'^2 - y'^2\rangle\}$, the Hamiltonian for the cubic field is diagonal, $H_{cub} = diag(E_{Od}, E_{Ot}, E_{Ot}, E_{Ot}, E_{Od})$, where $E_{Od}$ and $E_{Ot}$ denote the shift in energy of respectively the orbital doublet and triplet compared to the free $d$ electron.

At some lattice sites the cubic field has a trigonal distortion, which means that the cubic symmetry is reduced to a $C_{3v}$ symmetry with the $C_{3v}$ axis along a body diagonal of the cubic field, or the direction of the distortion. An adequate basis set for this particular crystal field is the set $cb = \{|z^2\rangle, |xz\rangle, |yz\rangle, |xy\rangle, |x^2-y^2\rangle\}$, where the $z$-axis is parallel to the $C_3$ rotational axis. This particular symmetry splits the degeneracy of the states in $cb$ into two orbital doublets and a singlet. The sets of cubic harmonics $\{|xz\rangle, |yx\rangle\}$ and $\{|xy\rangle, |x^2-y^2\rangle\}$, respectively, make up the orbital doublets, whereas the $\{|z^2\rangle\}$ corresponds to the orbital singlet. Thus, in the basis $cb$, the Hamiltonian for the trigonal field is $H_{trig} = diag(E_{C0}, E_{C1}, E_{C1}, E_{C2}, E_{C2})$, where $E_{C0}$, $E_{C1}$ and $E_{C2}$ denote the shift in energy of respectively the orbital singlet and doublets compared to the free $d$ electron.

It is useful to take the basis states with the spin of the electron included. A convenient basis set is the direct product of spherical harmonics and spin states. Let $sb = \{|2\rangle, |1\rangle, |0\rangle, |-1\rangle, |-2\rangle\}$ be a basis in terms of spherical harmonics where $|m\rangle$ denotes the spherical harmonic $Y_2^m$. The basis we use is then $\{sb\,|\uparrow\rangle, sb\,|\downarrow\rangle\}$, where $|\uparrow\rangle$ and $|\downarrow\rangle$ denote the electron spin projection along the $z$-axis. In order to transform $H_{cub}$ and $H_{trig}$ to this basis, the cubic harmonics need to be transformed to spherical harmonics, and $H_{cub}$ also needs to be rotated from the primed to the unprimed basis. The transformation from cubic to spherical harmonics is given by equations (s1) to (s5). The rotation from the primed to unprimed basis can be described by the three Euler angles $\alpha$, $\beta$ and $\gamma$, around the $z$, $x$, and $z$ axis respectively in this particular order. This rotation is described by $\beta = \arccos\big(1/\sqrt{3}\big)$ and $\gamma = \frac{3}{4}\pi$. The angle $\alpha$ has no effect on the direction of $z$-axis. However, choosing $\alpha = 0$ results in the simplest Hamiltonian. The rotation of spherical harmonics can be done by using the Wigner D matrix with these Euler angles. After $H_{cub}$ and $H_{trig}$ have been transformed to the basis $sb$, the total Hamiltonian can be written in block-diagonal form by reordering the basis states. The matrix blocks are

$$\mathcal{H}_1 = \mathcal{H}_2 = \begin{bmatrix} \frac{1}{3}(3E_{C2}+E_{Od}+2E_{Ot}) & -\frac{\sqrt{2}i}{3}(E_{Od}-E_{Ot}) & 0 \\ \frac{\sqrt{2}i}{3}(E_{Od}-E_{Ot}) & +\frac{1}{3}(3E_{C1}+2E_{Od}+E_{Ot}) & 0 \\ 0 & 0 & E_{C0}+E_{Ot} \end{bmatrix} \tag{s6}$$

$$\mathcal{H}_3 = \begin{bmatrix} \frac{1}{3}(3E_{C1}+2E_{Od}+E_{Ot}) & \frac{\sqrt{2}i}{3}(E_{Od}-E_{Ot}) & 0 & 0 \\ -\frac{\sqrt{2}i}{3}(E_{Od}-E_{Ot}) & \frac{1}{3}(3E_{C2}+E_{Od}+2E_{Ot}) & 0 & 0 \\ 0 & 0 & \frac{1}{3}(3E_{C2}+E_{Od}+2E_{Ot}) & -\frac{\sqrt{2}i}{3}(E_{Od}-E_{Ot}) \\ 0 & 0 & \frac{\sqrt{2}i}{3}(E_{Od}-E_{Ot}) & \frac{1}{3}(3E_{C1}+2E_{Od}+E_{Ot}) \end{bmatrix} \tag{s7}$$

with corresponding basis states

$$\mathcal{H}_1 : \Big( |2\rangle\,|{\uparrow}\rangle\,,\ |{-1}\rangle\,|{\uparrow}\rangle\,,\ |0\rangle\,|{\downarrow}\rangle \Big) \tag{s8}$$

$$\mathcal{H}_2 : \Big( |{-2}\rangle\,|{\downarrow}\rangle\,,\ |1\rangle\,|{\downarrow}\rangle\,,\ |0\rangle\,|{\uparrow}\rangle \Big) \tag{s9}$$

$$\mathcal{H}_3 : \Big( |1\rangle\,|{\uparrow}\rangle\,,\ |{-2}\rangle\,|{\uparrow}\rangle\,,\ |2\rangle\,|{\downarrow}\rangle\,,\ |{-1}\rangle\,|{\downarrow}\rangle \Big) \tag{s10}$$

The matrix blocks $\mathcal{H}_1$ and $\mathcal{H}_2$ are the same, and both have in general three distinct eigenvalues. This means that for each eigenstate of $\mathcal{H}_1$ there is an eigenstate of $\mathcal{H}_2$ with the same energy. Combined, $B_1$ and $B_2$ describe three doublets. The matrix block $\mathcal{H}_3$ has only 2 distinct eigenvalues and therefore describes 2 doublets, meaning that all eigenstates of the total Hamiltonian are at least doubly degenerate. This is in accordance to Kramers theorem, which states that for systems with half integer spin and time-reversal symmetry every state is at least doubly degenerate. When the nuclear spin is not included, the two electronic-spin states in a doublet are each others time-conjugate. This is indeed the case for our system.

## II. EFFECT OF VARYING PARAMETER $k$

In order to restrict the parameter range that we use to model the V defects in SiC at the $\alpha$ site, we look at regions where the model reproduces the experimental $g$-parameters and the spin-orbit splitting between ground state KDs. This agreement can be obtained for $k$ values between 0.18 and 0.37. The $k$ value has a strong influence on the relative trigonal crystal field strength $\eta$, but not on the SOC parameter $\lambda$ (figure S1). Figures S2(a-d) and S2(e-f) show the magneto-spectra obtained for the parameters corresponding to figures S1(a) and S1(b), respectively. The qualitative shape of the spectra does not change significantly when we consider different values of $k$, and neither does the order of magnitude of the Rabi frequencies obtained. We note, however, that lower $k$-values (which consequently require a larger trigonal crystal field) result in lower Rabi frequencies due to interactions with electric fields parallel to the crystal c-axis, and magnetic fields perpendicular to this direction.

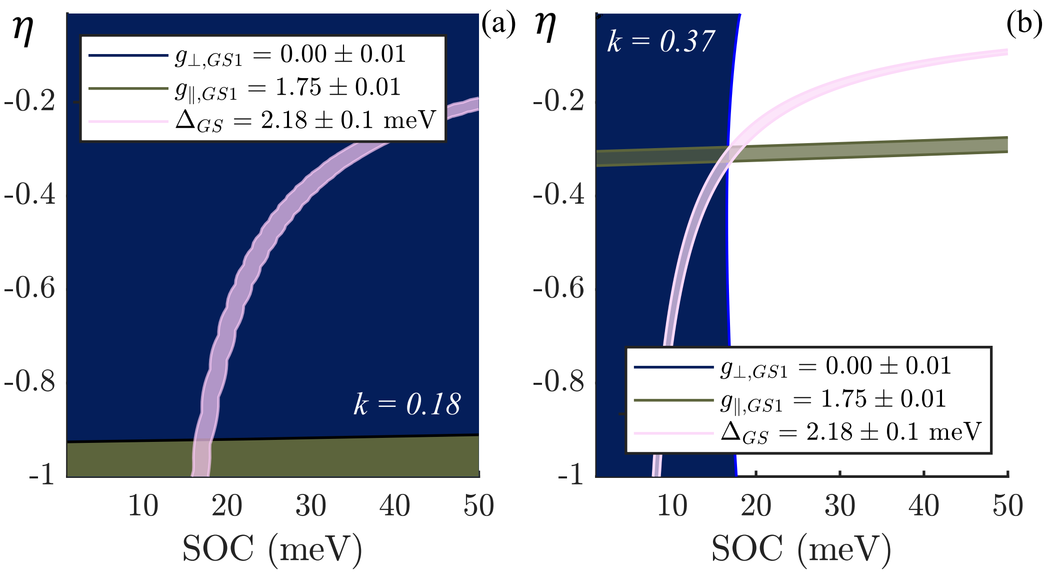


FIG. S1. Effect of varying the parameter $k$ on parameters $\eta$, $\lambda$ that match experimental observations. Values of $k$ between 0.18 (panel S1(a)) and 0.37 (panel S1(b)) provide parameter ranges that describe the experimental results well. Low $k$ values require stronger trigonal crystal fields (larger $\eta$). In contrast, the value of the SOC parameter ($\lambda$) does not depend strongly on the value of $k$.

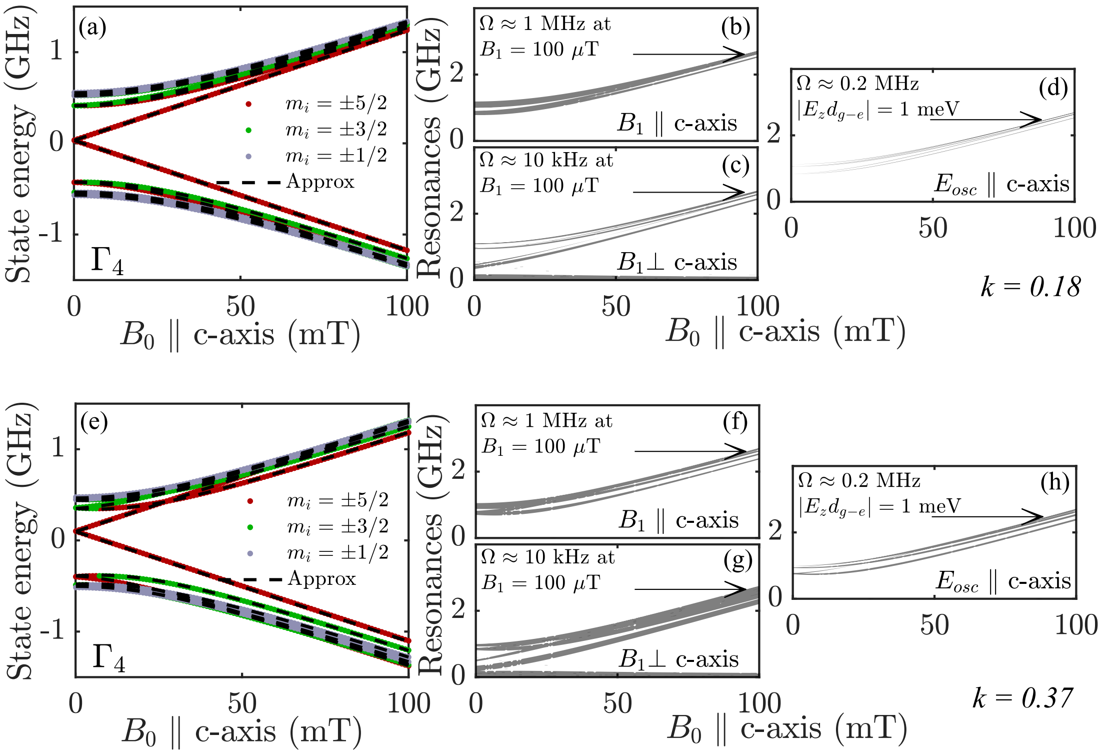


FIG. S2. Effect of varying the parameter $k$ on magneto-spectra of the $\Gamma_4$ doublets. Results are as presented in the main text for figure 3. We use the parameter range determined in figure S1(a) to obtain the plots in panels S2(a-d), and the parameters corresponding to figure S1(b) to obtain the plots in panels S2(e-f).

## III. ENERGY EIGENSTATES AND ALLOWED RESONANCES FOR $\Gamma_{5,6}$ DOUBLET

We can numerically obtain the results presented in figure 3 of the main text for the ground-state $\Gamma_{5,6}$ doublet. The shape of the magneto-spectrum differs from what figure 3 of the main text presents for the $\Gamma_4$ doublet. Figure S3 shows that, for the $\Gamma_{5,6}$ doublet there are no levels whose energy increases purely linearly with the applied magnetic field. This is the most striking feature, and would be visible in magnetic resonance spectra. Additionally, the spacing between the hyperfine levels is larger and more clearly resolved than for the $\Gamma_4$ doublet. Finally, for the $\Gamma_{5,6}$ states, the anticrossing points occur at finite magnetic fields for some of the hyperfine sublevels. All of these features can be used to identify the experimentally observed lowest-energy doublet as being of the $\Gamma_4$ type.

Finally, we note that the $\Gamma_{5,6}$ doublet in the $\alpha$ site is 2.18 meV above the lowest energy KD, such that its equilibrium population will be reduced at cryogenic temperatures according to the Boltzmann factor. Nonetheless, a weak signal of these states' spin properties may be visible at intermediary temperatures, where $k_B T \approx \Delta_{SOC}$. We note that, for the $\Gamma_{5,6}$ doublets, electronic magnetic resonance with oscillating fields perpendicular to the c-axis (figure S3(c)) is not possible due to the symmetry restricted $g_\perp = 0$. Only nuclear magnetic resonance lines are present in this case, at very low frequencies. Nonetheless, electronic magnetic resonance with an oscillating field along the symmetry axis of the defect remains possible (figure S3(d)).

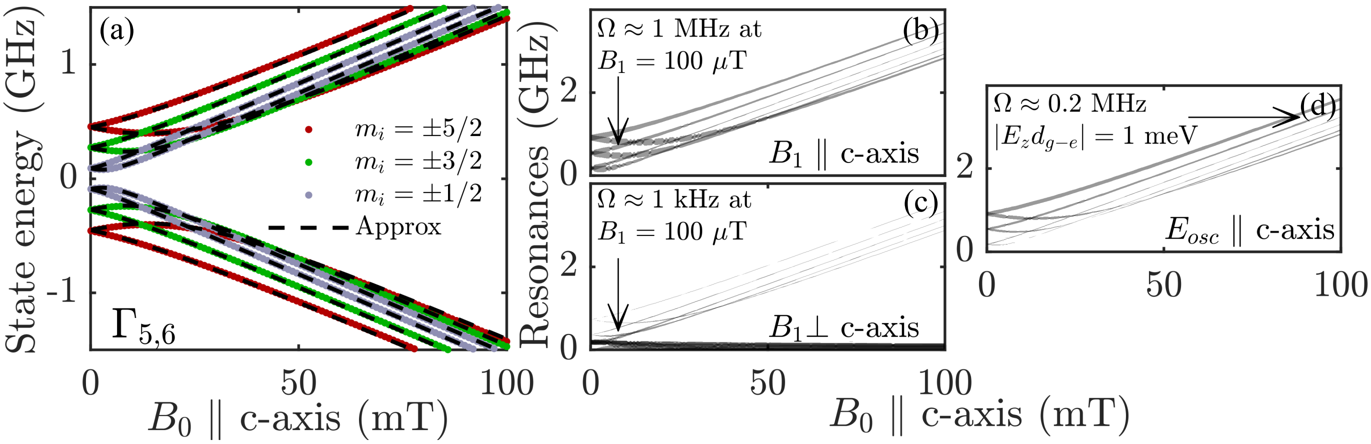


FIG. S3. (a) Energies of the 12 eigenstates corresponding to the $\Gamma_{5,6}$ ground-state electronic spin doublet, hyperfine-coupled to a central nucleus with a spin-5/2, as a function of the static magnetic field $B_0$ applied parallel to the c-axis. Results were obtained numerically (colored lines), and by diagonalizing the effective spin Hamiltonian associated with a $\Gamma_{5,6}$ doublet (dashed line). (b-d) Microwave resonance lines obtained numerically for an oscillating magnetic field parallel (b) or perpendicular (c) to the c-axis, or an oscillating electric field parallel (d) to the c-axis. The thickness of the resonance lines corresponds to their Rabi frequencies, with different scales in each figure. Scales are provided by the labels and arrows, indicating the Rabi frequency at a certain point. (b) If the static field is small (Zeeman splitting comparable to hyperfine coupling strength), a small oscillating magnetic field ($B_1 \approx 100$ $\mu$T) parallel to the c-axis leads to very efficient electronic spin transitions with Rabi frequencies on the order of 1 MHz. These resonances weaken significantly as the static magnetic field increases. (c) In a $\Gamma_{5,6}$ doublet, direct interaction with an oscillating field perpendicular to the c-axis is symmetry forbidden, such that electronic spin transitions are fully forbidden for fields in this direction. Only nuclear spin transitions are observed in this case. (d) A large enough electric field parallel to the c-axis mixes ground and optically excited states and deforms the electron density, modulating the influence of the anisotropic dipolar hyperfine coupling, which can result in electronic spin transitions.

## IV. MATRIX REPRESENTATION OF INTERACTION WITH ELECTRIC FIELDS

We obtain the matrix representation of the effect of an oscillating electric field by investigating the matrix elements of a trigonal crystal field as in equations (s6, s7), with

$E_{Od} = E_{Ot} = 0$ and $E_{C2} - E_{C_1} = E_{C0} = 1$ meV. We use, as basis states, the $|\Gamma_i, \uparrow\downarrow\rangle$ as defined in the main text (see caption of figure (2) in the main text).

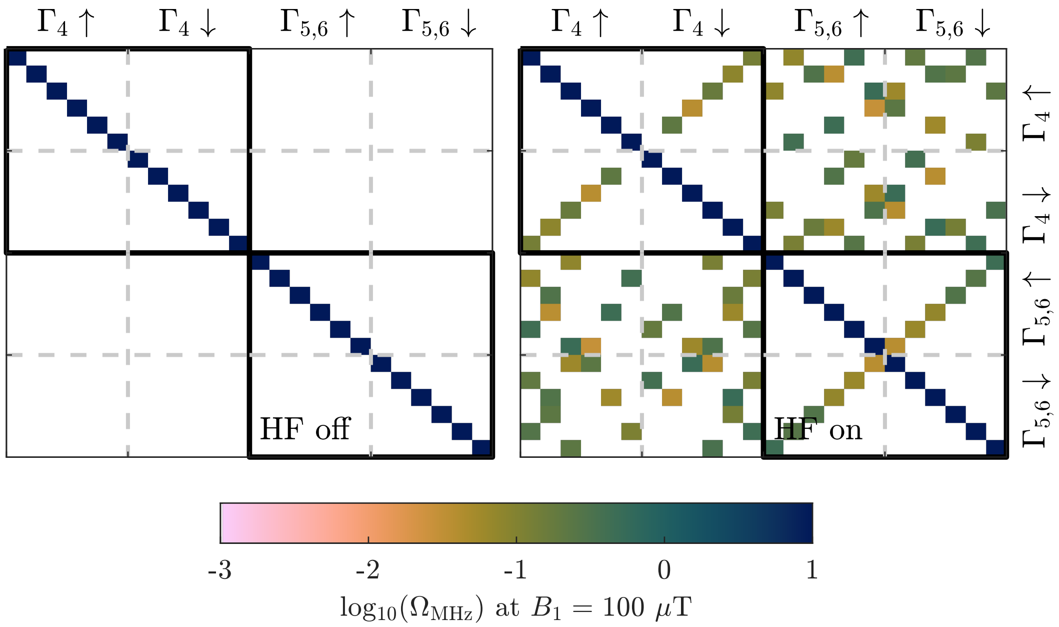


FIG. S4. (a) Matrix elements due to an oscillating electric field parallel to the c-axis, in the basis defined by the crystal field, spin-orbit coupling and a small magnetic field (20 mT) along the c-axis, for the two ground state Kramers doublets ($|\Gamma_4, \uparrow\downarrow\rangle$ and $|\Gamma_{5,6}, \uparrow\downarrow\rangle$), without hyperfine coupling. White matrix elements correspond to zero. Within each KD (contoured block diagonal parts of the full matrix), an electric field parallel to the c-axis does not lead to electric microwave transitions, consistent with the restrictions from Kramer's theorem [2, 3]. (b) Same as (a), but with the hyperfine interaction between electron and the central nuclear spin added to the static Hamiltonian. In this case, the electronic spin can flip via electric microwave transitions driven by an oscillating field parallel to the c-axis.

## V. RESULTS FOR V DEFECT IN $\beta$ SITE

In 4H-SiC, V can occupy two different lattice sites, which gives rise to defects with distinct optical transitions and electronic configurations [4–7]. The $\alpha$ site is subject to the strongest trigonal crystal field and shows the largest values for spin-orbit splitting between the two ground-state KDs. We base our analysis in the main text on this lattice site, since it is most similar to the recently explored Mo defects [2, 8]. Nonetheless, we can repeat the procedure

of the main text for the $\beta$ site as well, which we present here. Figure S5 shows that in order to reproduce the experimentally observed energy splittings for the ground state of these defect centers, we need to take much weaker trigonal fields ($\eta = -0.2$ for the $\beta$ site, versus $\eta = -0.4$ for the $\alpha$ site, with the same value of $k$). Also the spin-orbit parameter $\lambda$ is reduced from 17 meV in the $\alpha$ site to ~5 meV in the $\beta$ site.

Although the hyperfine spectra obtained with these parameters are qualitatively similar to those shown in the main text for the $\alpha$ defect, there are some differences that are worth noting. At large magnetic fields, the energies of the hyperfine sublevels of the $\Gamma_4$ doublet are more closely spaced (figure S6(a)), giving rise to magneto-resonance spectra where the hyperfine lines are less clearly distinguishable (figure S6(b-d)). This may have consequences for experimental schemes that rely on being able to resolve these spin transitions and address them independently. Additionally, we note that for the $\Gamma_{5,6}$ KD of the V defect in the $\beta$ configuration, electronic spin transitions due to oscillating magnetic fields perpendicular to the symmetry axis of the defect arise (figure S6(g)). This is in contrast to what figure S3(c) presents for the $\alpha$ site. In the $\beta$ site, since the SOC splitting between ground-state doublets is small, a magnetic field perpendicular to the symmetry axis can mix the $\Gamma_4$ and $\Gamma_{5,6}$ doublets. This causes that the symmetry protection with regards to spin transitions due to oscillating magnetic fields perpendicular to the c-axis observed for the $\alpha$ site is not effective at the $\beta$ site.

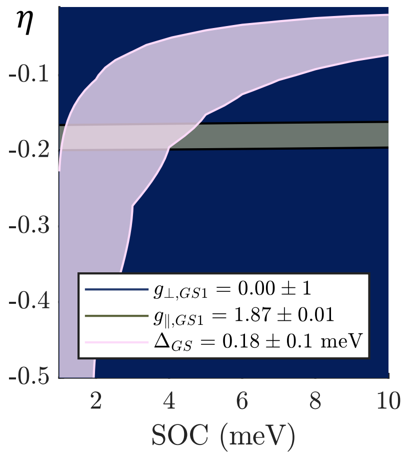


FIG. S5. Parameters that reproduce the ground-state energy splittings of a $\beta$-site V defect in 4H-SiC [5], for $k = 0.3$.

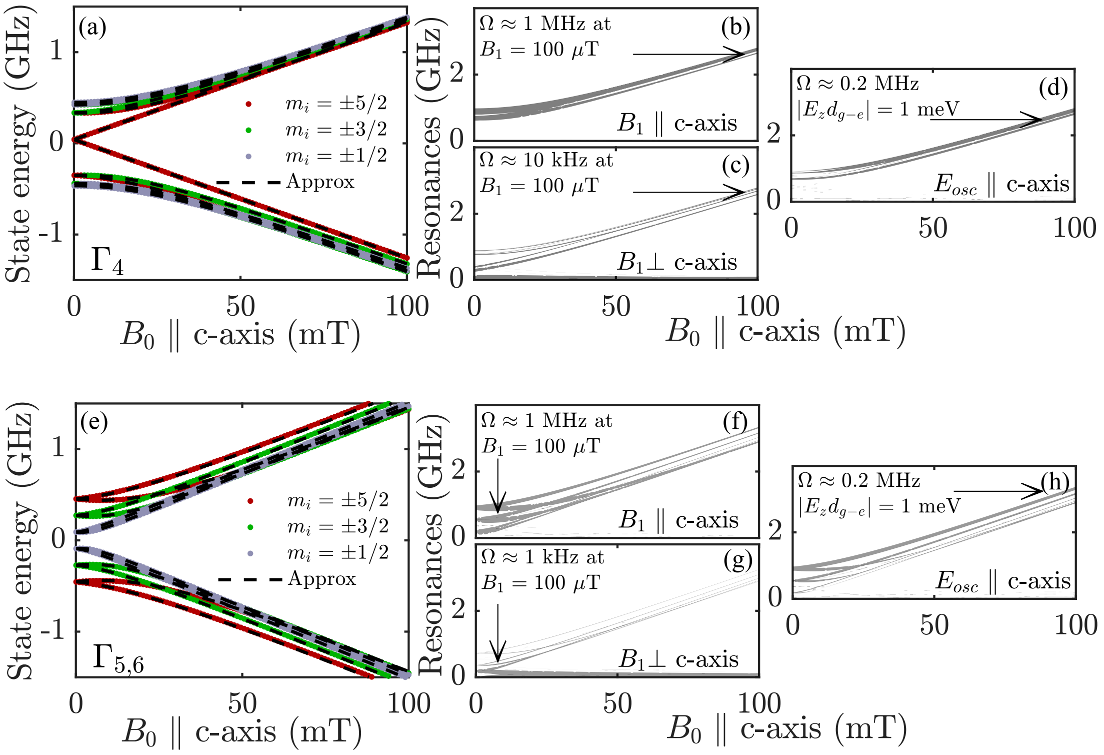


FIG. S6. Hyperfine level structure and allowed microwave transitions of the $\Gamma_4$ (a-d) and $\Gamma_{5,6}$ (e-h) doublets with parameters as obtained in figure S5.

## VI. ANALYTICAL EXPRESSIONS FOR EFFECTIVE-SPIN HAMILTONIAN

In order to obtain analytical expressions for the effective-spin Hamiltonians, we diagonalize the Hamiltonians in equations (s6, s7) algebraically. To do this, we parametrize the terms $E_{Od,Ot}$ and $E_{C0,C1,C2}$, such that

$$\Delta = E_{Ot} - E_{Od} \tag{s11}$$

$$\Delta_E = E_{C1} - E_{C2} = \eta\Delta \tag{s12}$$

$$\epsilon_{Td} = (E_{Ot} + E_{Od})/3 \tag{s13}$$

$$\epsilon_{C3} = (E_{C1} + E_{C2}) \tag{s14}$$

and pick $\epsilon_{Td}$, $\epsilon_{C3}$ such that the energies are centered at zero.

This results in a crystal-field Hamiltonian in terms of the parameters $\eta$, $\Delta$ and $\Delta_A$ (as defined in the main text)

$$B_1 = B_2 = \Delta \begin{bmatrix} -\frac{1}{2}(\eta-\frac{1}{3}) & \frac{\sqrt{2}i}{3} & 0 \\ -\frac{\sqrt{2}i}{3} & \frac{1}{2}(\eta-\frac{1}{3}) & 0 \\ 0 & 0 & E_{C0}+E_{Ot} \end{bmatrix} \tag{s15}$$

$$B_3 = \Delta \begin{bmatrix} \frac{1}{2}(\eta-\frac{1}{3}) & -\frac{\sqrt{2}i}{3} & 0 & 0 \\ \frac{\sqrt{2}i}{3} & -\frac{1}{2}(\eta-\frac{1}{3}) & 0 & 0 \\ 0 & 0 & \frac{1}{3}-\frac{1}{2}(\eta-\frac{1}{3}) & \frac{\sqrt{2}i}{3} \\ 0 & 0 & -\frac{\sqrt{2}i}{3} & \frac{1}{2}(\eta-\frac{1}{3}) \end{bmatrix} \tag{s16}$$

Within the ground state manifold, composed by the lowest-energy $\Gamma_4$ and $\Gamma_{5,6}$ doublets, this Hamiltonian has eigenstates [3, 9]

$$|\Gamma_4^g, \uparrow\rangle = \sin(\phi)\,|2, \uparrow\rangle + i\cos(\phi)\,|{-1}, \uparrow\rangle \tag{s17}$$

$$|\Gamma_4^g, \downarrow\rangle = \sin(\phi)\,|{-2}, \downarrow\rangle + i\cos(\phi)\,|1, \downarrow\rangle \tag{s18}$$

$$\left|\Gamma_{5,6}^g, \uparrow\right\rangle = \sin(\phi)\,|{-2}, \uparrow\rangle + i\cos(\phi)\,|1, \uparrow\rangle \tag{s19}$$

$$\left|\Gamma_{5,6}^g, \downarrow\right\rangle = \sin(\phi)\,|2, \downarrow\rangle + i\cos(\phi)\,|{-1}, \downarrow\rangle \tag{s20}$$

in terms of the parameter

$$\phi = \text{atan}\left(\frac{2\sqrt{2}}{1 - 3\eta + 3\sqrt{1 + \eta^2 - \frac{2}{3}\eta}}\right) \tag{s21}$$

The parameter $\phi$ thus indicates the relative strengths of the trigonal and tetrahedral crystal fields. For $\eta = 0$, where there is no trigonal component in the crystal field, $\phi = 35.26^o$. In contrast, if the trigonal contribution is much larger than the tetrahedral contribution, $\eta = \pm\infty$, such that $\phi = 90^o$ and $\phi = 0^o$, respectively. In these latter cases, the eigenstates fully coincide with the spherical harmonics with the $z$-axis along the $C_3$ symmetry axis.

In order to obtain the analytical expressions for the effective-spin Hamiltonians presented in the main text, we include spin-orbit coupling to first order. That is, we assume that the SOC energy splitting is big enough to isolate the KDs $\Gamma_4^g$ and $\Gamma_{5,6}^g$ from each other, but disregard the effect of SOC in mixing ground and optically excited-state doublets. We then write the Hamiltonians corresponding to the Zeeman energy and the hyperfine interaction in the basis given by $\{\left|\Gamma_{4,(5,6)}, \uparrow\downarrow, m_i\right\rangle\})$, where $m_i$ corresponds to the nuclear spin projection along the $z$-axis.

We obtain the effective-spin Hamiltonians presented in the main text,

$$H_{\Gamma_4} = H^{eff}_{\mathrm{HF}} + H^{eff}_{\mathrm{Zee,el}} + H^{eff}_{\mathrm{Zee,nuc}} \tag{s22}$$

$$H^{eff}_{\mathrm{HF}} = a_{\parallel,\Gamma_4}\tilde{S}_z I_z + a_{\perp,\Gamma_4}(\tilde{S}_+ I_+ + \tilde{S}_- I_-) \tag{s23}$$

$$H^{eff}_{\mathrm{Zee,el}} = -\mu_B\big(g_{\parallel,\Gamma_4} B_z \tilde{S}_z + g_{\perp,\Gamma_4}(B_x\tilde{S}_x + B_y\tilde{S}_y)\big) \tag{s24}$$

$$H^{eff}_{\mathrm{Zee,nuc}} = -\mu_N g_n\big(B_z I_z + B_x I_x + B_y I_y\big) \tag{s25}$$

$$H_{\Gamma_{5,6}} = H^{eff}_{\mathrm{HF}} + H^{eff}_{\mathrm{Zee,el}} + H^{eff}_{\mathrm{Zee,nuc}} \tag{s26}$$

$$H^{eff}_{\mathrm{HF}} = (a_{\parallel,\Gamma_{5,6}}\tilde{S}_z + a_{\perp,\Gamma_{5,6}}\tilde{S}_y)I_z \tag{s27}$$

$$H^{eff}_{\mathrm{Zee,el}} = -\mu_B g_{\parallel,\Gamma_{5,6}} B_z \tilde{S}_z \tag{s28}$$

$$H^{eff}_{\mathrm{Zee,nuc}} = -\mu_N g_n\big(B_z I_z + B_x I_x + B_y I_y\big) \tag{s29}$$

with parameters

$$\Gamma_4 \begin{cases} a_\parallel & = \frac{2}{7}A(7k-1)(3\sin^2(\phi)-1) \\ a_\perp & = \frac{6}{7}A\cos^2(\phi) \\ g_\parallel & = 2(k(3\sin^2(\phi)-1)+1) \\ g_\perp & = 0 \end{cases} \tag{s30}$$

$$\Gamma_{5,6} \begin{cases} a_\parallel & = \frac{2}{7}A(7k+1)(3\sin^2(\phi)-1) \\ a_\perp & = \frac{6}{7}A\sin(2\phi) \\ g_\parallel & = 2(-k(3\sin^2(\phi)-1)+1) \\ g_\perp & = 0 \end{cases} \tag{s31}$$

with parameteres $A$, $k$ as defined in the main text. A first-order correction to the wave-functions due to spin-orbit coupling modifies $g_\perp$ for the $\Gamma_4$ doublet, giving rise to a small non-zero $g_\perp$ on the order of $(k\lambda/\Delta)$. This does not happen for the $\Gamma_{5,6}$ doublet.

To obtain these values, we have relied on the fact that the hyperfine coupling and the Zeeman interaction with the magnetic fields are both much smaller than the spin-orbit related energy splitting between the KDs. This is valid in the case of the $\alpha$ site. For the $\beta$ and $\gamma$ sites, where the SOC splitting is smaller, mixing between the $\Gamma_4$ and $\Gamma_{5,6}$ KDs due to

magnetic fields and interaction with the nuclear spin become relevant, and the validity of these effective-spin-1/2 Hamiltonians in describing the energy levels and allowed transitions is limited.

---


[1] A. Gällström, B. Magnusson, and E. Janzén, "Optical identification of Mo related deep level defect in 4H and 6H SiC," Materials Science Forum **615**, 405 (2009).

[2] C. M. Gilardoni, T. Bosma, D. van Hien, F. Hendriks, B. Magnusson, A. Ellison, I. G. Ivanov, N. T. Son, and C. H. van der Wal, "Spin-relaxation times exceeding seconds for color centers with strong spin–orbit coupling in SiC," New J of Phys **22**, 103051 (2020).

[3] B. Tissot and G. Burkard, "Spin structure and resonant driving of spin-1/2 defects in SiC," Phys Rev B **103**, 064106 (2021).

[4] B. Kaufmann, A. Dörnen, and F. S. Ham, "Crystal-field model of vanadium in 6H silicon carbide," Phys Rev B **55**, 13009 (1997).

[5] G. Wolfowicz, C. P. Anderson, B. Diler, O. G. Poluektov, F. J. Heremans, and D. D. Awschalom, "Vanadium spin qubits as telecom quantum emitters in silicon carbide," Sci Adv **6**, eaaz1192 (2020).

[6] L. Spindlberger, A. Csóré, G. Thiering, S. Putz, R. Karhu, J.Ul Hassan, N.T. Son, T. Fromherz, A. Gali, and M. Trupke, "Optical properties of vanadium in 4H silicon carbide for quantum technology," Phys Rev Applied **12**, 014015 (2019).

[7] J. Baur, M. Kunzer, and J. Schneider, "Transition metals in SiC polytypes, as studied by magnetic resonance techniques," Phys Stat Sol A **162**, 153 (1997).

[8] T. Bosma, G. J. J. Lof, C. M. Gilardoni, O. V. Zwier, F. Hendriks, B. Magnusson, A. Ellison, A. Gällström, I. G. Ivanov, N. T. Son, R. W. A. Havenith, and C. H. van der Wal, "Identification and tunable optical coherent control of transition-metal spins in silicon carbide," npj Quantum Information **4**, 48 (2018).

[9] A. Csóré and A. Gali, "*Ab initio* determination of pseudospin for paramagnetic defects in SiC," Phys Rev B **102**, 241201(R) (2020).
